# Supplementary material for: Radically Lower Data-Labeling Costs for Visually Rich Document Extraction Models
Source: arXiv:2210.16391 source file (2022-10-28)
Supplement: Supplementary file 1 [file supplementary.tex]

\clearpage
\section{Response to Reviewer Comments}
\vspace{5pt}
\subsection{Meta Reviews}
\vspace{-5pt}
\reviewerquestion{
%\begin{reviewerquote}
Thank you for your submission to PVLDB 2023. We have now received the reviews for your manuscript from the Review Board. As you can see from the reviews themselves, the reviewers in general like the idea and effectiveness of the approach, and also the way in which the paper is written, but still have some concerns, therefore we are unable to accept the paper as it is but advise a revision, based on the revision items.
Your paper stimulated the interest of the reviewers, since it addresses a timely and interesting problem. However, the reviewers feel that the paper, even if generally well-written, lacks discussion or explanation on some very important points, such as: (i) the way the system is bootstrapped, (ii) a more precise explanation of the hypothesis made and of the parameters used, (iii) comments on the generalizability of the approach, (iv) clearer explanations of the annotation assumptions and method, and of the process of imperfect candidate generation, and (v) the need of a (from various viewpoints) richer experimental campaign.
You will find many more useful details in the reviews themselves, especially in the Weak Points and Detailed Comments.} 
%\end{reviewerquote}

We’d like to thank the reviewers for their thoughtful comments and suggestions. These have helped us make the paper substantially stronger and clearer. Below is a summary of the changes we’ve made. Detailed responses to each of the reviewer’s questions follow, along with a pointer to the section we modified in response:
\begin{itemize}
    \item Expanded Section~\ref{sec:assumptions} to include discussion on imperfect candidate generators.  
    \item Revised Section~\ref{sec:selective_labeling_uncertainty} to explain the parallel between score distance metric and entropy-based metric. Also improved Section~\ref{sec:calibration} to clearly describe the score calibration method.
    \item Expanded Section~\ref{sec:setup}, added Table~\ref{tab:parameter} to present our hyperparameter choices. Briefly explained the relationship between the candidate generator recall and the extraction recall. Also added a footnote to describe how we count the number of questions to ask according to the annotation budget.  
    \item Edited Section~\ref{sec:perfield} and Section~\ref{sec:conclusion} to explain how this technique is effective even with imperfect candidate generators.
    \item Expanded Section~\ref{sec:relatedwork} to  discuss relationship with crowdsourcing literature. 
\end{itemize}

\subsection{Reviewer \#1}
\vspace{-5pt}
%\begin{reviewerquote}
\reviewerquestion{Q1: How is the model bootstrapped?}
%\end{reviewerquote}

The model is bootstrapped by randomly selecting a small number of documents (50-250, which is much smaller than the pool of ~10K unlabeled documents) and labeling them using the classic annotation workflow. The binary classifier-based model is trained on this small set of fully labeled documents and used for iteratively selecting candidates for annotation thereafter.

%\begin{reviewerquote}
\reviewerquestion{Q2: While I appreciate the authors listing all the assumptions, I would like to see more justification of each of those assumptions.}
%\end{reviewerquote}

In Section~\ref{sec:assumptions}, we list four assumptions: (1) a pool of unlabeled documents is accessible; (2) the extraction model can be trained on partially labeled documents; (3) the model can generate candidate spans for measuring the uncertainty; and (4) annotating a 25-field document takes 6 minutes and answering a yes/no question takes 10 seconds. (1) is easy to justify -- many companies are manually processing such documents and have access to a pool of unlabeled documents they bring when trying to evaluate automatic document processing solutions from Cloud vendors like Google, Microsoft, and Amazon. The motivation for adopting these automatic processing solutions is the volume of these documents they need to process -- labels are the scarce resource here.  We justify (2) and (3) empirically in this paper - we showed that it is possible to extend the binary classifier in \citep{majumder2020representation} to train on partially labeled documents effectively, and simply re-use the candidate-generation machinery of \citep{majumder2020representation} and use the binary classifier to compute uncertainty scores. The detailed discussion can be found in Figure~\ref{fig:glean} and Section~\ref{sec:assumptions}. Finally, in addition to evidence from \citep{cloudresearchblog} to justify the assumption (4), we acquired stats from our team of annotators on how long the classic annotation takes for various document types. We found it averaged 6-8 min for an annotator to label a single-page document with fewer than 20 fields while it averaged 10-30 min for an annotator to label a multi-page document with 25 fields. So we picked a very conservative value (6 min) as the estimated time of labeling one document in this paper. 

%\begin{reviewerquote}
\reviewerquestion{
Q3: Unclear description of parameters and how they are set. How was the annotation budget determined? How is the field-specific threshold parameter decided? Overall, setting up values for the parameters is one of the biggest challenges. There are other parameters such as m (Sec 3.3). I would like to see a list of parameters (preferably a table) and mechanism to choose these parameter values.}
%\end{reviewerquote}

Yes, setting up proper values for hyperparameters is challenging. We apply grid search to find the most performant values (to maximize F1 scores) on a development dataset for all the hyperparameters including m and k’ in Section~\ref{sec:selective_labeling_sampling}. We reorganized the details and added them to Table 2. The annotation budget is computed based on the time needed to annotate a full document and to answer a yes/no question. For example, it takes 6 min/doc * 10k docs = 3.6M seconds to label the full unlabeled dataset with the classic annotation workflow. We regard this duration as the 100\% annotation cost, 10\% of which equals a 0.36M-second budget, and at 10 seconds per yes/no question, this gives us a budget of 36k questions. If we bootstrap the model using the classic annotation workflow on 100 documents, we simply subtract that cost from the 0.36M-second budget for selective annotation. The budget is fixed at 10\%, but varies across datasets of different sizes when translated to the number of yes/no questions. Following the common practice used in prior art, the field-specific thresholds we describe in Section~\ref{sec:assumptions} are also determined by finding the thresholds that maximize F1 scores for each field on a development set.

%\begin{reviewerquote}
\reviewerquestion{Q4: The uncertainty measures are ad-hoc. Can an entropy-based uncertainty model work here?  Section 3.2.1 (score calibration) seems ad-hoc as well. I would think all these depend on the dataset or domain of the problem. Is the proposed approach generalizable for other domains (different kinds of documents) and different problems (e.g., weak supervision)?}
%\end{reviewerquote}

Yes, an entropy-based uncertainty model works. In fact, in the binary classification task, the entropy-based solution: $x^{*}=\underset{x}{\arg\max} -P(y=0|x)\text{log}P(y=0|x)-P(y=1|x)\text{log}P(y=1|x)$ finds candidates with scores closest to 0.5, which is identical to our score distance method. We updated the text in Section~\ref{sec:selective_labeling_uncertainty} to clarify this.

Regarding score calibration, neural networks are often poorly calibrated regardless of dataset or domain~\citep{guo2017calibration}. There are many methods for model calibration, including Platt scaling and histogram binning~\citep{platt1999probabilistic,naeini2015obtaining,ZadroznyE01,ZadroznyE02}. We use a modified version of histogram binning~\citep{ZadroznyE01} and ISORegC~\citep{ZadroznyE02} which is most useful in scenarios with large class imbalances. However, we expect that any calibration method that deals with skewed distributions would work. We updated Section~\ref{sec:calibration} to clarify this. 

%\begin{reviewerquote}
\reviewerquestion{Q5: One tradeoff here is whether one should focus on achieving better accuracy for "easy" fields or "difficult" fields. I suppose easy fields can be improved by fewer annotations and difficult ones might require more annotated data. On the other hand, we have to strike a balance between frequent and rare fields. Fields that occur more frequently should have more accuracy. How do these two orthogonal dimensions interact for the proposed system?}
%\end{reviewerquote}

This is a really interesting question. Empirically, we found that ``difficulty'' and ``frequency'' are not entirely orthogonal. (If we use accuracy as a proxy for difficulty, rarer fields tend to have lower F1 scores.) However, in this paper, we do not explicitly differentiate between fields based on difficulty or frequency.  Since we are optimizing for macro F1, which weighs each field equally irrespective of frequency, we let the selection algorithm focus on uncertainty. Macro F1 is the typical goal for most extraction applications. If on the other hand, we were optimizing for Micro F1 (F1 computed across all instances, not average across all fields), focusing on improving frequent fields may be better -- perhaps by using a combination of uncertainty and frequency to guide the process by which we select candidates for yes/no questions.

%\begin{reviewerquote}
\reviewerquestion{Q6: I suppose each field is annotated by multiple annotators. One important factor here is annotator trustworthiness. This could be a crucial factor in achieving correct ground truth.}
%\end{reviewerquote}

Yes, for all the document types, we follow the procedure where every document is labeled by an annotator, and then sent to a designated expert annotator who reviews the annotations to guarantee data quality.  We agree this is a critical factor in achieving correct ground truth. In a few cases, we still notice incorrect annotations while surprisingly, we find that selective labeling has the potential to mitigate the impact (details explained in Q7).

%\begin{reviewerquote}
\reviewerquestion{Q7: I would like to see experiments with varying target accuracy. Say to achieve a fixed accuracy k, how much annotation is needed by the proposed approach and baselines. A model to measure user effort and show user effort and accuracy gain ratio would be an interesting experiment.}

%\end{reviewerquote}
We gradually increased the annotation budget and observed the corresponding results in Table~\ref{tab:budgets}. 
\begin{table}[t]
    \centering
    \resizebox{\linewidth}{!}{
    \begin{tabular}{c|c|c|c|c|c|c|c}
        \hline
        & \multirow{2}{*}{Cost} & \multicolumn{2}{c|}{Supplier Chain} & \multicolumn{2}{c|}{Retail Finance}  & \multicolumn{2}{c}{Tax Forms}  \\
        \cline{3-8}
        & &  F1 & gap closed &  F1 & gap closed &  F1 & gap closed \\
        \hline
        \hline
        \multirow{4}{*}{SL} & 0\% & 0.547 & 0.0\% & 0.644 & 0.0\% & 0.773 & 0.0\% \\ 
         & 10\% & 0.687 & 88.6\% & 0.678 & 91.9\% & 0.836 & 88.7\% \\ 
         & 20\% & 0.704 & 99.4\% & 0.682 & 102.7\% & 0.844 & 100.0\% \\ 
         & 30\% & 0.706 & 100.6\% & 0.686 & 113.5\% & 0.845 & 101.0\% \\ 
        \hline
        FL & 100\% & 0.705 & 100.0\% & 0.681 & 100.0\% & 0.844 & 100.0\% \\ 
        \hline
    \end{tabular}
    }
    \vspace{5pt}
    \caption{Comparisons of the extraction performance and gap closed by SL when consuming different annotation costs on three datasets. SL 0\%, 10\%, and FL 100\% corresponds to the Initial, Selective Labeling, and Full Labeling stats in Figure~\ref{fig:domains}. (SL: Selective Labeling, FL: Full Labeling)}
    \label{tab:budgets}
    \vspace{-20pt}
\end{table}
Here we compared the extraction performance and gap closed using 10\% (same as stats in Figure~\ref{fig:domains}), 20\%, and 30\% of the annotation budget. If our goal is to close the gap by about 90\%, then 10\% of the labeling cost is enough to achieve the goal (for all three data sets). If our goal is to close the gap by 99\%, then 20\% of the labeling cost is sufficient for three datasets. The performance of selective labeling can even exceed the full labeling setup (see results for 30\% of the labeling cost). We believe that’s because the algorithm avoids selecting a few incorrect annotations that can confuse the model especially when the model has already determined predictions with low uncertainty that are contrary to the ground-truth annotation. We already hit the page-limit, so unfortunately, we 
could not add this table to the paper. 

\subsection{Reviewer \#2}
\vspace{-5pt}
%\begin{reviewerquote}
\reviewerquestion{Q1: This paper reminds me of papers in the crowdsourcing line of work, where a goal is to minimize/simplify questions to the crowdworkers. The additional dimension, considered in some crowdsourcing work and not in this paper, is the quality of crowdworkers. That is, one could send more complex questions to higher-quality crowdworkers and simpler questions to lower-quality crowdworkers. It will be interesting to see what the authors have in mind regarding this aspect or whether they always think they can simplify the questions to yes/no questions. Some discussion on this front will be of interesting additional value to the paper, I think.}

%\end{reviewerquote}
Thank you for bringing up this line of work! The crowdsourcing literature was indeed one of the sources of inspiration for this work. We cited  related papers and expanded this  discussion in Section~\ref{sec:relatedwork}. Crowdsourcing and selective labeling do have similarities, such as seeking annotators to answer questions to achieve high-quality labeled data. Our goal in this work is not to measure/understand annotator quality, but to argue for structuring the labeling task in a way that imposes a low cognitive burden, and modify the ML to make it dramatically cheaper to acquire labeled data. For now, all the questions can be simplified to the same “Yes/No” format such as “Is candidate A a correct value for field B in this document?”. We believe this format not only reduces the cognitive burden from all the annotators but also eases the estimation of annotation cost. But yes, as we explore asking annotators to do more complex tasks like correcting pseudo-labels or re-drawing bounding boxes (see discussion in Section~\ref{sec:conclusion}), we will draw from the ideas in the crowdsourcing literature for efficient annotation assignment. 

\subsection{Reviewer \#3}
\vspace{-5pt}
%\begin{reviewerquote}
\reviewerquestion{Q1: Seems to skip over the issue of imperfect candidate generation, which is the primary reason why one does full document manual annotation
\begin{itemize}
    \item In general for these types of IE problems, if you trusted the candidate generation process to be 100\% recall (i.e. cover all actual extractions with generated candidate set), then you would of course label at the candidate level (and could apply active learning as is standard).
    \item However, the reason full-document annotation is generally done is because other than for very simple extraction types (e.g. numbers, dates), candidate generation is *not* perfect
    \item The paper seems to skip this major point entirely- unless I am missing something and/or misunderstanding the method employed.
    \item If so: the paper (A) is extremely opaque about the proposed approach's central limitation, and (B) the proposed approach is both less novel and less generally applicable (i.e. I would guess mostly applicable to simple entity types e.g. numbers, dates)
\end{itemize}}
%\end{reviewerquote}

We fully agree with the reviewer that the problem of imperfect candidate generation requires more discussion. We build on the architecture in \citep{majumder2020representation,tata2021glean} where they have already demonstrated that high-recall candidate generators can be built (and are in use) for many fields like numbers, prices, dates, names of people, places, organizations, (using canned named-entity annotators) addresses (using canned address detectors), alphanumeric strings (canned regexes), etc. We denote the recall of candidate generation as coverage (to distinguish this from recall of extractions) and present this for a few fields in the table below. For simple fields, this is indeed in the 90s (\textit{date\_of\_delivery}, \textit{purchase\_order}), but for other fields it is lower. Having a candidate generator with low recall indeed limits the recall of the final extractions and therefore the final F1 score for that field. A key contribution of this paper is that even with imperfect candidate generation, that is, on fields with low candidate coverage, selective-labeling allows us to deliver big improvements to the final extraction F1 score for that field. See F1 scores before and after selective labeling for fields in the Supply Chain dataset in Table~\ref{tab:coverage}. 

\begin{table}[hb]
    \centering
    \resizebox{\linewidth}{!}{
    \begin{tabular}{c|c|c|c|c}
        \hline
        Field & CG Recall & F1 w/o SL & F1 w/ SL & $\Delta$ \\
        \hline
        \hline
        \textit{date\_of\_delivery} & 0.932 & 0.690 & 0.759 & 10.00\% \\
        \textit{purchase\_order} & 0.992 & 0.884 & 0.963 & 8.94\% \\
        \textit{customer\_address} & 0.484 & 0.293 & 0.363 & 23.89\% \\
        \textit{customer\_name} & 0.715 & 0.526 & 0.621 & 18.06\% \\
        \hline
    \end{tabular}
    }
    \vspace{5pt}
    \caption{The F1 performance comparison between w/o Selective Labeling and w/ Selective Labeling on four fields. (CG Recall: Candidate Generator Recall)}
    \label{tab:coverage}
    \vspace{-15pt}
\end{table}
For simple extraction types such as \textit{purchase\_order} (numbers) and \textit{date\_of\_delivery} (dates), selective labeling can improve their extraction performance by ~10\%, thanks to high candidate generation coverage. For fields with low candidate generation coverage such as customer name and customer address, selective labeling is still able to find the uncertain candidates and dramatically improve their extraction F1 by 24\% and 18\% respectively. We added text in Section~\ref{sec:perfield} explaining that selective labeling is effective even when candidate generators are far from perfect. 
We agree with the reviewer that adapting selective labeling to models that do not require candidate generation at all would be an interesting line of work. We added to this discussion in Section~\ref{sec:conclusion} -- there are several open questions around how to accomplish this. This is indeed ongoing work with strong preliminary results. A full discussion is beyond the scope of this paper, and we expect to publish those results in a follow-on work.

Finally, we would like to respectfully point out that even with perfect candidate generation (100\% recall), naively using candidate-level labeling (yes/no questions) instead of the classic annotation workflow ends up being more expensive. As we explain in Section~\ref{sec:proposed_annotation_workflow}, this is  because we typically see dozens of candidates for many fields, and answering yes/no for each of these candidates ends up taking longer than the classic annotation workflow.

%\begin{reviewerquote}
\reviewerquestion{Q2: Lack of clarity as to evaluation of candidate generation accuracy
\begin{itemize}
    \item Are the scores generated over a candidate set generated by the automatic candidate generator and then labeled, or over the actual ground truth? I.e. Do the reported scores take into account candidate generator errors?
    \item This is somewhat unclear in the presentation.
    \item Again, this is important, because the main reason to do full doc annotation is to handle imperfections in candidate generation. Either the paper is restricted to studying a simpler subset of the extraction landscape where this is not an issue, or I was just confused by the presentation.
\end{itemize}}

%\end{reviewerquote}
All F1 scores are generated by comparing the extractions with the \textbf{ground truth}. If a field has a poor candidate generator (say \textit{customer\_address}), its final recall can obviously not exceed the recall of the candidate generator. Per request, we have made it clear in the paper (Section~\ref{sec:setup}). Thanks for pointing out this confusion. 

%\begin{reviewerquote}
\reviewerquestion{Q3: Somewhat simple method + somewhat small set of evaluations
\begin{itemize}
    \item If judged on methodological novelty: as per above, labeling candidates + using active learning is not novel.
    \item If judged on scope of empirical evaluation: I would expect more datasets / extraction and entity types.
\end{itemize}}

%\end{reviewerquote}
We think simplicity is actually one of the advantages of our annotation framework, making this particularly suitable for practical deployment. We do not claim any advances to the state-of-the-art in active learning: our contribution focuses on scaling the acquisition of labeled data for a rapidly growing set of document-processing products cheaply through a novel combination of simple active-learning and data science techniques. We are the first to show a dramatic reduction of annotation cost by customizing this idea to the document extraction field (which is currently bottle-necked by annotation costs). We have tested the algorithm on a wide range of datasets – Supply Chain, Retail Finance, and Tax Forms, containing 18, 11, and 24 entity types respectively (as shown in Table~\ref{tab:datasets}). We see strong evidence that the selective labeling algorithm can generalize well to other document types.
